# Supplementary material for: The role of Coulomb interaction in superconducting NbTiN thin films
Source: arXiv:1711.04585 source file (2017-11-13)
Supplement: Supplementary file 1 [file Supplimentary_NbTiN_Superconductivity_arxiv.tex]

\documentclass[aps,showpacs,amsmath,amssymb,twocolumn,final]{revtex4-1}

\usepackage{graphicx, epstopdf}

\begin{document}

\title{Supplemental Material: \\ The role of Coulomb interaction in superconducting NbTiN thin films}

\author{D. Hazra$^{1}$, N. Tsavdaris$^{2}$, A. Mukhtarova$^{1}$, M. Jacquemin$^{2}$, F. Blanchet$^{1}$, R. Albert$^{1}$, S. Jebari $^{1}$, A. Grimm$^{1}$, E. Blanquet$^{2}$, F. Mercier$^{2}$, C. Chapelier$^{1}$ and M. Hofheinz$^{1}$}

\affiliation{$^{1}$ Univ.\ Grenoble Alpes, CEA, INAC-Pheliqs, 38000 Grenoble, France }
\affiliation{$^{2}$ Univ.\ Grenoble Alpes, CNRS, Grenoble INP, SIMaP,  38000 Grenoble, France}

\email []  {iamdibyenduhazra@gmail.com}

\date{\today}

\maketitle

Determination of $\xi (0)$ : 

The zero temperature Ginzburg-Landau coherence length ($\xi (0)$) is estimated from $\xi(0)= \sqrt{\Phi_0/2\pi \,T_c \left|\frac{dB_{c2}}{dT}\right|_{\,T=\,T_c}} $ \cite{tinkham1996introduction}. For that, magnetoresistance data are collected for all the samples up to a magnetic field of 8\,T. In Fig. \ref{fig:Magres}a, we show the magnetoresistance data for S1, where temperature variation of $\rho_{xx}$ is recorded at five different fields. $B_{c2}(\,T)$ is determined as the point where $\rho_{xx}$ is half of the normal resistivity. In Fig. \ref{fig:Magres}b, we plot $B_{c2}$ as a function of temperature. The solid lines are straight line fits. The slopes and the $\xi(0)$ are listed in Table-\ref{fig:Magres}.

\setcounter{figure}{0}
\renewcommand{\thefigure}{S\arabic{figure}}
\begin{figure}\centerline{\includegraphics[width=9cm,angle=0]{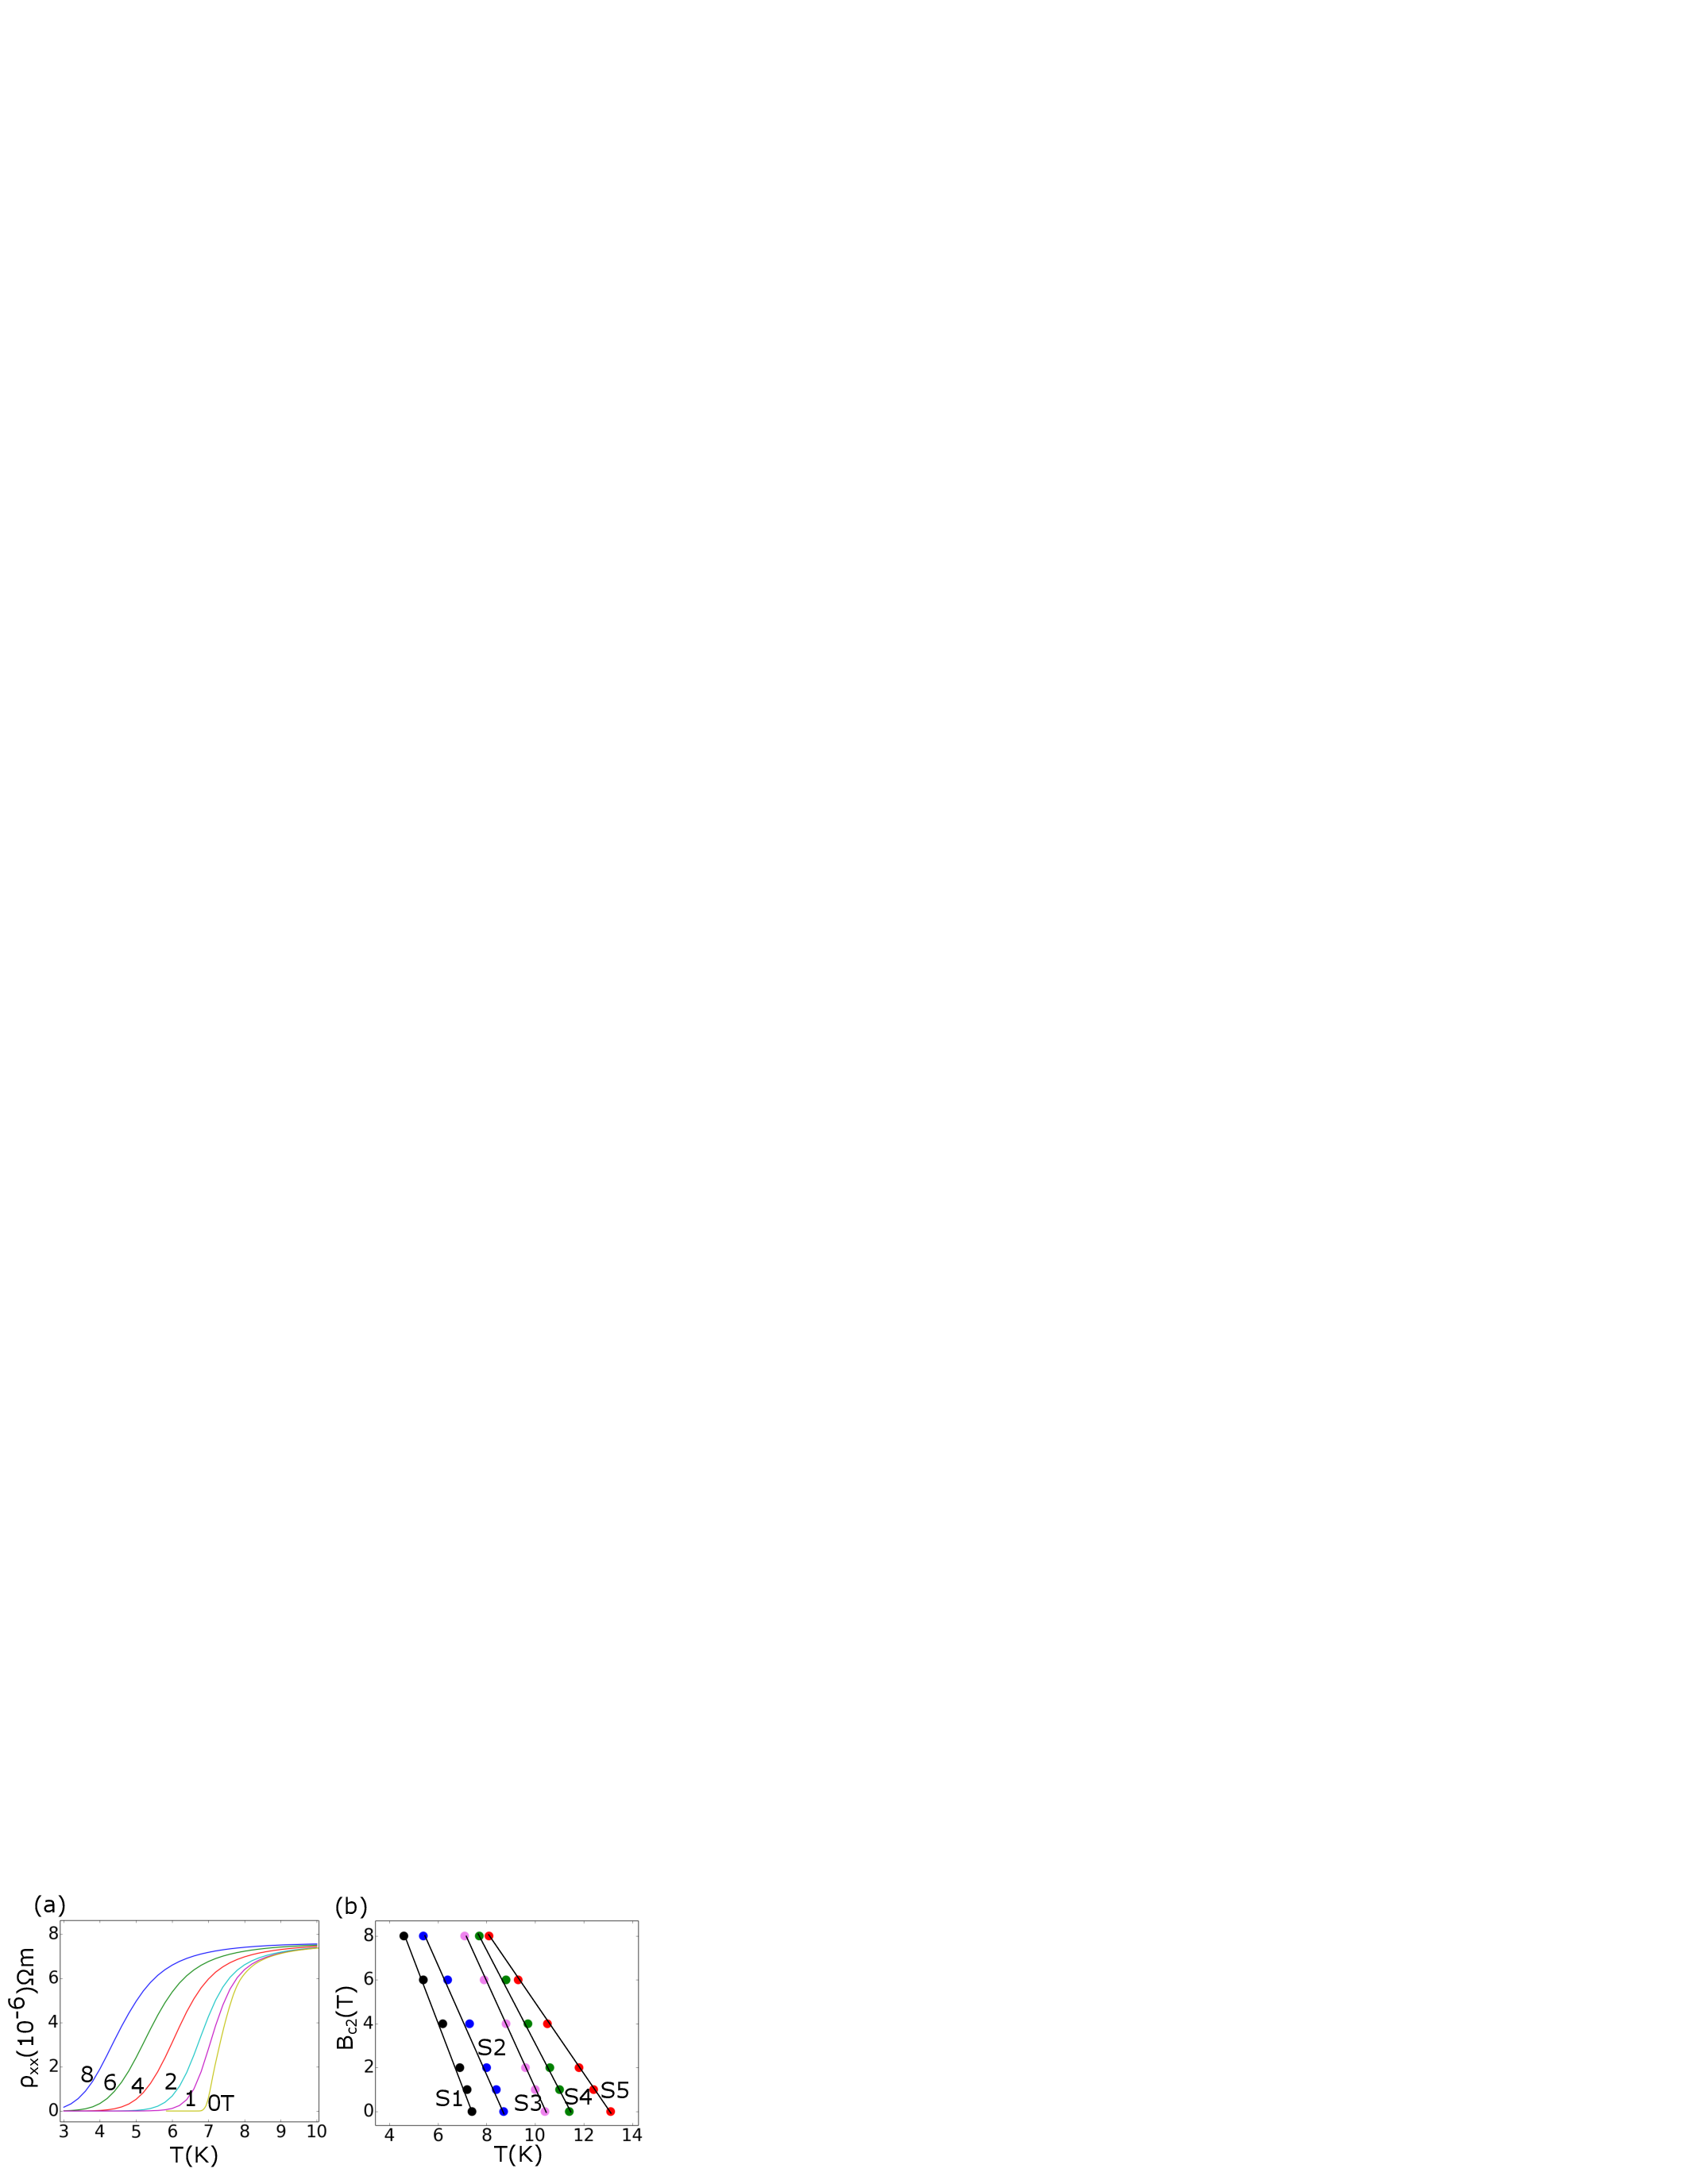}}
	\caption {(a) Temperature dependence of $\rho_{xx}$ for S1 at different magnetic fields as indicated in the figure. (b) The variation of $B_{c2}$ as a function of temperature for all five samples. The solid lines are straight line fits.}
	\label{fig:Magres}
\end{figure}

\setcounter{table}{0} 
\renewcommand{\thetable}{S\arabic{table}}
\begin{table}
	\caption{\label{tab2} $ \left|\frac{dB_{c2}}{dT}\right|_{\,T=\,T_c} $ and $\xi$(0) of our $\mathrm {Nb_{1-x}Ti_xN}$ thin films.   }
	\begin{tabular}{|c|c|c|}
		\hline
		Samples & $ \left|\frac{dB_{c2}}{dT}\right|_{\,T=\,T_c} $ &  $\xi$(0)    \\
		
		& (\,T/\,K) & (nm) \\  \hline
		
		S1       &3.23 & 6.1 \\
		S2        &2.60&  5.8 \\
		S3        &2.41  & 5.5\\
		S4        &2.30  & 5.3  \\
		S5      & 1.60 &  5.8 \\
		
		\hline
	\end{tabular}
\end{table}

%\section{Error estimation}

%We could measure temperature within 50\,mK accuracy.  The thickness measurement and shape asymmetry, i.e, the imperfection in the Hall geometry are two main sources of errors, which are about 10\% and 5\%, respectively. They subsequently propagate error to other quantities--- $\rho_{xx}$,  $R_{H}$ and all the free electron parameters. As a result, the errors, for instances, in $\rho_{xx}$, $n$ and $k_{F} \ell$ are about 15\%, 10\%, and 12\%, respectively. 

\bibliography{Bibliography}
\end{document}
